# Supplementary material for: Peering inside the black box: Learning the relevance of many-body functions in Neural Network potentials
Source: arXiv:2407.04526 source file (2024-07-05)
Supplement: Supplementary file 1 [file SI.pdf]

# Peering inside the black box: Learning the relevance of many-body functions in Neural Network potentials

Klara Bonneau[1†], Jonas Lederer[2,3†], Clark Templeton[1*†], David Rosenberger[1], Klaus-Robert Müller[2,3,4,5*], Cecilia Clementi[1,6,7*]

[1]Department of Physics, Freie Universität Berlin, Arnimallee 12, 14195, Berlin, Germany.
[2]Machine Learning Group, Technische Universität Berlin, Marchstr. 23, 10587, Berlin, Germany.
[3]BIFOLD - Berlin Institute for the Foundations of Learning and Data, Germany.
[4]Department of Artificial Intelligence, Korea University, Korea University, Seoul, 136-713, South-Korea.
[5]Max Planck Institute for Informatics, 66123, Saarbrücken, Germany.
[6]Center for Theoretical Biological Physics, Rice University, Houston, 77005, TX, USA.
[7]Department of Chemistry, Rice University, Houston, 77005, TX, USA.

*Corresponding author(s). E-mail(s): clarktemple03@gmail.com; klaus-robert.mueller@tu-berlin.de; cecilia.clementi@fu-berlin.de;
†These authors contributed equally to this work.

# S1 Simulation Details

## S1.1 All-Atom Simulations

### S1.1.1 Water & Methane

As reference data for the water and methane models, we use atomistic (AA) simulations with a periodic methane or TIP3P water box containing 125/258 atoms respectively. Only the heavy atoms were retained under the CG coordinate mapping: C for methane and O for water. All simulations were run in OpenMM [1] with Langevin dynamics at a temperature of 300K controlled with a damping coefficient of 1 $ps^{-1}$. Each system was simulated for 50 ns using a 1 fs timestep with both coordinates and forces saved every 1 ps. These coordinates and forces (or delta-forces, see below) are what are used in training the neural network model using force matching. The water box was initiated using the openmmtools [2] testsystem `WaterBox` with parameter `box_edge` = 2 nm. The methane box was created using topotools [3] and simulated using the parameters in Table S1.

| | |
|---|---|
| $q_C$ = -0.36e | $q_H$ = 0.09e |
| $\epsilon_C$ = 0.326 $\frac{kJ}{mol}$ | $\epsilon_H$ = 0.100 $\frac{kJ}{mol}$ |
| $\sigma_C$ = 0.339 nm | $\sigma_H$ = 0.239 nm |
| $k_{bond}$ = 269450 $\frac{kJ}{mol \cdot nm^2}$ | $r_0$ = 0.111 nm |
| $k_{angle}$ = 297 $\frac{kJ}{mol \cdot rad^2}$ | $\theta_0$ = 1.89 rad |

**Table S1** Methane Parameters for simulation in the AA system. Parameters are given for partial charges of Carbon and Hydrogen, LJ interactions, and bond & angle parameters.

### S1.1.2 NTL9

The data used for the fast-folding variant of NTL9 (PDB ID 2HBA) is part of the dataset used in the previous study by Majewski et. al. [4]. For convenience, the relevant details are briefly summed up here. NTL9 was solvated and ionized in a cubic box of side length 50Å as in Ref. [5]. ACEMD [6] and GPUGRID [7] were used to run MD

| | Water & Methane | NTL9 |
|---|---|---|
| Integrator | Langevin | Langevin |
| Friction | 1 $ps^{-1}$ | 1 $ps^{-1}$ |
| Timestep | 5 fs | 2 fs |
| Temperature | 300K | 350K |
| Number of steps | 40000 | $4 \times 10^6$ |
| Masses | Atomistic | Atomistic |

**Table S2** Parameters for simulation of the CG models of the different systems.

simulations of the system using the CHARMM22star force-field [8] and the TIP3P water model [9] at 350K. For production runs, a Langevin integrator with a timestep of 4fs and a friction damping constant of $0.1ps^{-1}$ was used. Hydrogen to heavy atom bonds were holonomically constrained with 4 times hydrogen masses [10]. An MSM-based adaptive sampling approach [11] was used to enhance the sampling efficiency. From a total of 256 $\mu$s aggregated simulation time, about 2.4 million frames were used for training and validation.

### S1.2 CG simulations

CG simulations were performed in the same way as Husic et. al. [12], using Langevin dynamics with the BAOA(F)B integration scheme. The specific parameters for each system are summed up in Table S2. Multiple independent simulations were run on a single GPU for efficient sampling.

## S2 Neural Network Training

Coarse-grained models were trained using the same CGSchNet approach introduced in previous studies [13, 12] but replacing the SchNet representation by equivariant models (PaiNN and SO3Net). In the CGSchNet approach, a thermodynamically consistent CG potential of mean force is learned via a reformulation of the force-matching approach [14, 15, 16] as a machine learning problem. The mapping operator for the

CG forces called ”basic aggregated” in [17] was chosen to be consistent with the presence of hydrogen-bond constraints in the training dataset. All training was done using SchNetPack 2.0 [18].

For water and NTL9, a delta-learning approach is used where the CG energy is decomposed into $U(\mathbf{R};\boldsymbol{\theta}) = U_{prior}(\mathbf{R}) + U_{net}(\mathbf{R};\boldsymbol{\theta})$, with $U_{prior}$ based on physical intuition and where only $U_{net}$ is learned during training. The goal is to prevent bad model extrapolation in unphysical regions of the configuration space, that inherently lack training data.

For water, only a repulsive prior between CG beads in the form $U_{rep}(r) = \phi(r) - \phi(r_{cut}) - (r - r_{cut})\frac{d\phi}{dr}|_{r=r_{cut}}$ with $\phi(r) = \left(\frac{\sigma}{r}\right)^{12}$ is used. Values of $\sigma$ and $r_{cut}$ are determined by inverting the probability distribution of two-particle distances. From this distribution, $\sigma$ is set at 0.05% of the closest distance, while $r_{cut}$ is chosen to correspond to the first detected peak. Values for $\sigma$ and $r_{cut}$ are 2.6 and 2.7 Å respectively.

For NTL9, the prior has the form $U_{prior}(\mathbf{R}) = \sum_{bonds} U_{bond}(r) + \sum_{angles} U_{angle}(\theta) + \sum_{dihedrals} U_{dihedral}(\phi, \psi) + \sum_{non-bonded} U_{rep}(r)$. Here, $U_{bond}$, $U_{angle}$ and $U_{dihedral}$ are the same as used in previous studies [17], but the repulsive prior is set to $U_{rep}(r) = k \times ReLU((\sigma - r)^3)$ with $k = 20 kcal/mol$ and $\sigma$ set to the minimum of the corresponding distribution in the training set, in order for its energy to be zero in the interpreted folded structures.

## S2.1 Training hyperparameters

All models were trained using the AdamW optimizer [19] with a learning rate of $5.10^{-4}$ and a weight decay coefficient of 0.01. The hyperparameters for the different models are given in Table S3.

| | Water & Methane PaiNN | Water & Methane SO3Net | NTL9 PaiNN |
|---|---|---|---|
| RBF type | Gaussian | Gaussian | Gaussian |
| RBFs | 15 | 20 | 20 |
| Atom. features | 128 | 128 | 128 |
| Int. blocks | 3 | 3 | 3 |
| Lmax | 1 | 2 | 1 |
| Cutoff | 7.5Å | 5Å | 10Å |
| Activation | SiLU | SiLU | Tanh |

**Table S3** Hyperparameters for the different models

# S3 Comparison with other models

## S3.1 Water & Methane

As a comparison to the PaiNN and SO3Net models shown in the main text, Fig. S1 shows the performance of the Inverse Monte Carlo (IMC) method and a SchNet [20] model on the same systems.

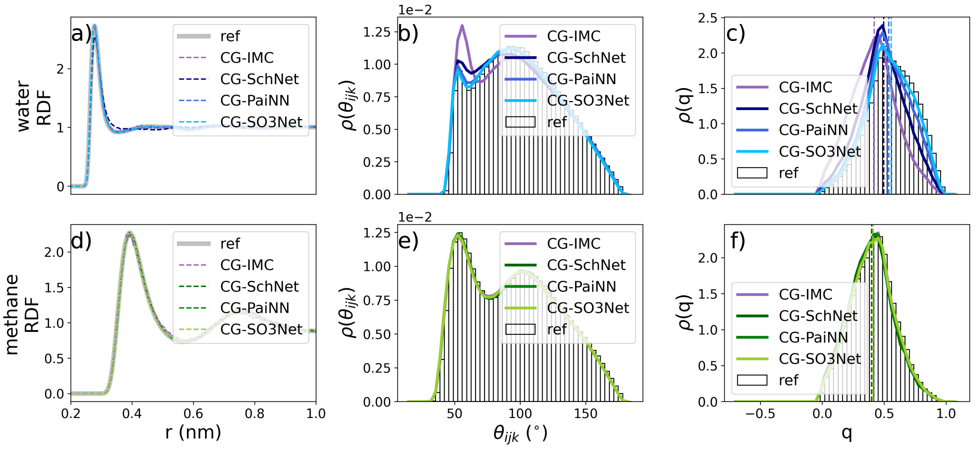


**Fig. S1** Performance of various CG models on water (top) and methane (bottom). In each row, the left plot shows the performance of the models on reproducing the RDF, the middle plot shows the local angle distribution and the right plot shows the tetrahedral order parameter as defined in Eq. (1). The dashed lines in panels c) and f) show the mean of the corresponding tetrahedral order parameter distribution.

IMC allows one to reconstruct pair potentials from known radial distribution functions (RDFs). This method shows the results that can be achieved on these systems with a 2-body only method.

SchNet can be considered as the predecessor of PaiNN, as it is a message-passing architecture with only invariant ($l_{\max} = 0$) features. It was trained on the atomistic reference data for water and methane in the same procedure as PaiNN and SO3Net. The hyperparameters for the shown SchNet water model are 64 Gaussian RBfs, 256 atomistic features, 6 interaction blocks, 10 Å cutoff, Tanh activation, and for the SchNet methane model 16 PhysNet-style RBFs, 128 atomistic features, 3 interaction blocks, 5 Å cutoff and Tanh activation.

Panels a) and d) of Fig. S1 show the RDFs obtained with all methods. IMC recovers the RDFs both for water and methane, unsurprising since the RDF was the optimization target of the method. Perhaps more interestingly, while for methane all models perform well, SchNet is not capable of fully recovering the RDF of water, whereas architectures incorporating equivariant features succeed in that attempt. We explain this by the fact that to compensate for the lack of equivariant features, SchNet may need a much larger cutoff than equivariant architectures to recover directional information crucial to the modelling of CG water. In our experiments, even with a 10 Å cutoff and six interaction blocks, SchNet cannot recover the RDF fully.

Panels b) and e) of Fig. S1 show the local angle distribution of the different CG models compared to the reference atomistic one. Local angle distributions are computed as the distribution of angles for triplets of beads located inside a cutoff [21, 22] set here to the end of the first solvation shell (3.5Å for water and 5.6Å for methane), i.e. for all triplets of beads $i$, $j$ and $k$ (considering all permutations), if $r_{ij} < r_{cut}$ and $r_{jk} < r_{cut}$, then $\theta_{ijk}$ is counted in the distribution. The angle distribution for methane in panel e) is very similar to the one of a Lennard-Jones fluid with preference for icosahedral packing corresponding to the sharp peak around 63° and the broader peak around 116°. In contrast, water (panel b) has a much stronger peak around 109.5° corresponding to the tetrahedral arrangement and a smaller peak around 50-60° corresponding to interstitial water molecules inside a tetrahedral arrangement. One can

see that while for methane all models recover the local angle distribution correctly, for water only the models including many-body terms capture the right overall shape and the inclusion of equivariant features makes the prediction quantitative.

To highlight the importance of the many-body terms further, panels c) and f) of Fig. S1 show the distribution of the orientational tetrahedral order, $q$, of the different CG models compared to the corresponding distribution in the reference atomistic model. The orientational order parameter is defined as

$$q = 1 - \frac{3}{8} \sum_{j=1}^{3} \sum_{k=j+1}^{4} \left( cos\, \theta_{jk} + \frac{1}{3} \right)^2 \tag{1}$$

where $\theta_{jk}$ is the angle formed by a given bead and its two nearest neighbors $j$ and $k$ [23, 24]. The value of $q$ can vary between -3 and 1 for an individual molecule and the average value for a collection of molecules ranges between 0 and 1 where 0 corresponds to an ideal gas structural arrangement, and 1 corresponds to a perfectly packed tetrahedron [24, 25]. Dashed vertical lines in panels c) and f) of Fig. S1 show the mean $\langle q \rangle$ value.

On panel f) of Fig. S1, one can see that the $q$ distribution for methane is very similar to the one of a Lennard-Jones system [24], driven by pairwise interactions with little to no many-body effects. In contrast, panel c) shows that the $q$ distribution for water has a more pyramid-like structure and displays a shoulder corresponding to transient arrangements shown to be stronger at low temperatures [24]. One can see that only the equivariant architectures PaiNN and SO3Net capture this behavior correctly, SchNet fails at reproducing the shoulder and IMC predicts a Lennard-Jones-like distribution.

These results show that for a complex system like bulk water, even if simple methods are correctly capturing the 2-body effects, higher-order features are needed to recover many-body observables.

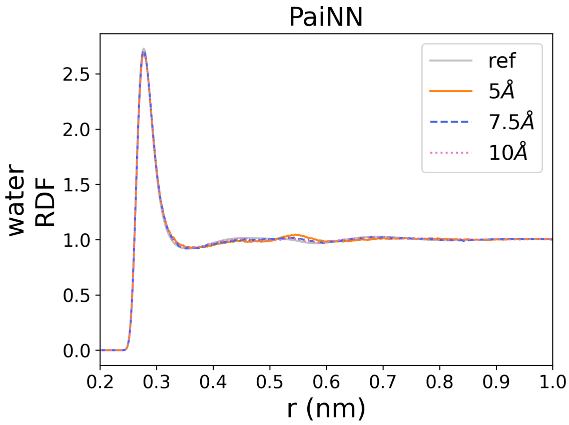


**Fig. S2** Performance of PaiNN water models with different cutoff radii. The RDF associated with different PaiNN models is shown in comparison to the all-atom reference RDF in grey. The agreement with the reference increases with increasing cutoff radius. In particular, PaiNN with a cutoff radius of 5 Å, does not reproduce the RDF well, while the improvement from 7.5 Å to 10 Å is negligible. Hence, we pick the PaiNN model with cutoff 7.5 Å for the entire analysis shown in the main text.

Figure S2 shows the performance of three PaiNN models with different network cutoffs. The model with a cutoff of 5 Å does not reproduce the RDF correctly. Increasing the cutoff to 7.5 Å corrects for this. Increasing the cutoff even further to 10 Å does not bring any substantial improvement and makes the relevance computation prohibitively expensive (by increasing drastically the total number of walks in the graph), which is why the 7.5 Å cutoff model was chosen for the analysis. For the SO3Net model shown in the main text, a 5 Å cutoff is enough to recover the structural features of the atomistic model.

# S4 Additional analysis

Figure S3 shows the distances corresponding to the most stabilizing or destabilizing interactions flagged by the network. For all systems and models, the lowest relevance values correspond to distances in the first solvation shell, deemed stabilizing by the models. Destabilizing interactions (high positive values) are located at distances too

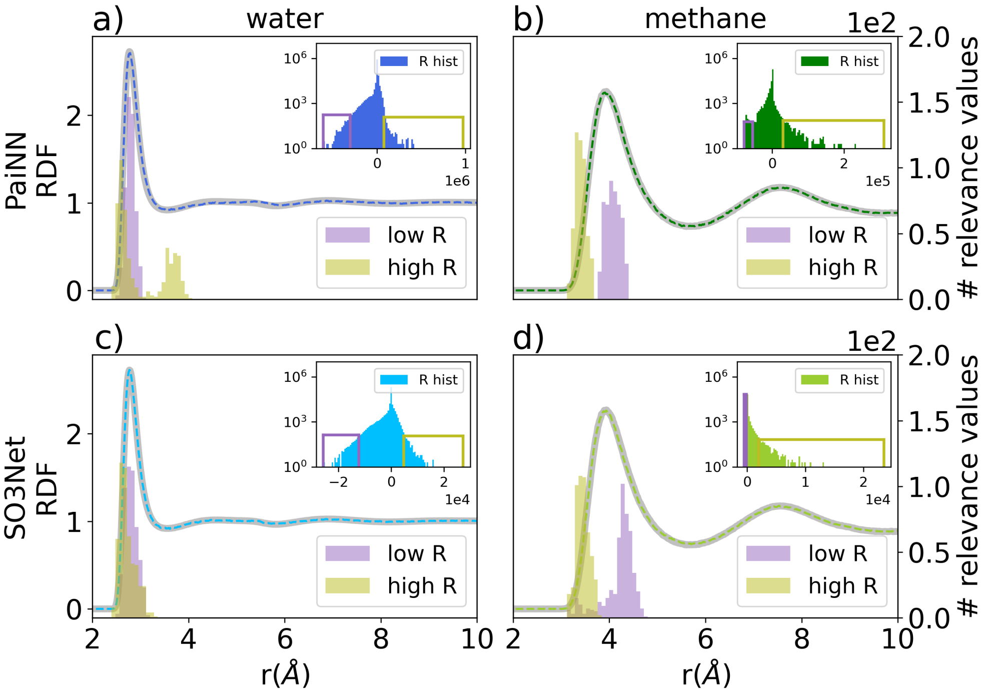


**Fig. S3** Highest and lowest 2-body relevances as a function of the distance. For each model and system, the distribution in distance of the 500 highest and lowest relevance values is plotted. As an inset is shown the entire distribution of two-body relevances.

short to be in the first solvation shell (rise of the RDF) and for PaiNN water (panel a) also for distances between the first and the second solvation shell.

Figure S4 shows the distances that have a zero relevance, i.e. that do not contribute to the network prediction. Reassuringly, one can see that these distances correspond exactly to the network cutoff in each case.

Figure S5 shows the three-body relevances divided into walks with and without self-loops as a function of the angle and distance. As also shown on Fig. 3 in the main text, the relevance of the three-body walks for methane is negligible compared to water. For water, it is interesting to observe that the relevance of the walks with self-loop varies much more as a function of the distance than the angle, indicating that these walks correct for the two-body contributions.

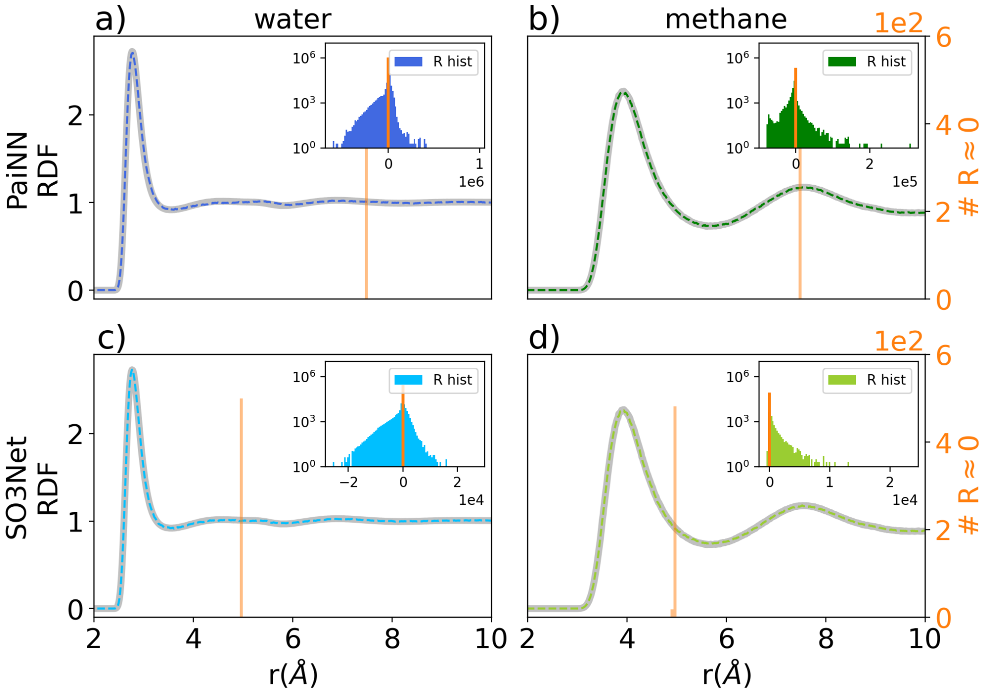


**Fig. S4** Zero two-body relevances as a function of the distance. The layout is the same as for Fig. S3.

Figure S6 shows the distances between residues in the interpreted structures for protein NTL9. Compared to panel a) of Fig. 5 in the main text, panel a) of Fig. S6 shows that PaiNN is capturing the interaction decay with the distance between residues. The comparison between panel b) of Fig. 5 in the main text and panels b) and c) of Fig. S6 shows that the 2-body interactions learned by the network between residues contain much more information than just pairwise distances, as they report on the stability of secondary structure elements inside the intermediate states.

# S5 Implementation of GNN-LRP

In this section we describe how the relevance attribution is obtained using efficient backpropagation under consideration of the respective propagation rules. Furthermore, it is explained in detail how relevance attributions are obtained for PaiNN and SO3Net.

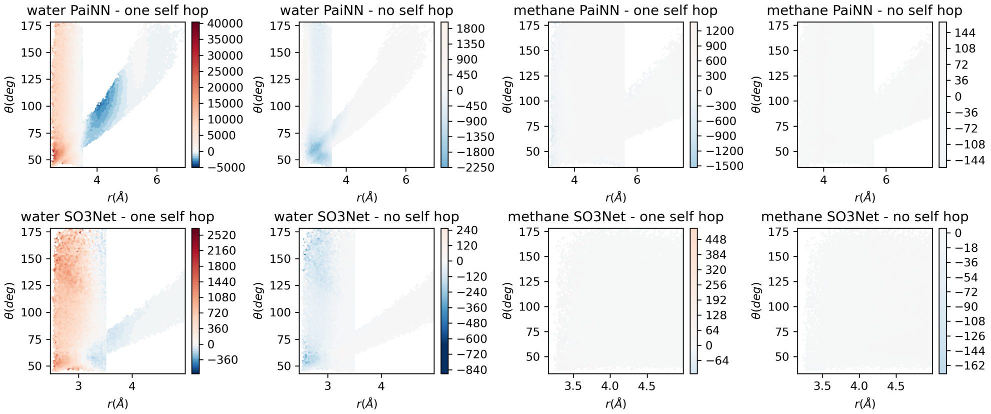


**Fig. S5** 3-body relevances within the first solvation shell as a function of their angle and distance. Colors show the relevance value, only triplets of water molecules inside the first solvation shell are considered, the angle plotted is the one between the two distances inside the first solvation shell (same as for the angle distribution, see above) and the distance plotted is the length of the edge opposite to the plotted angle.

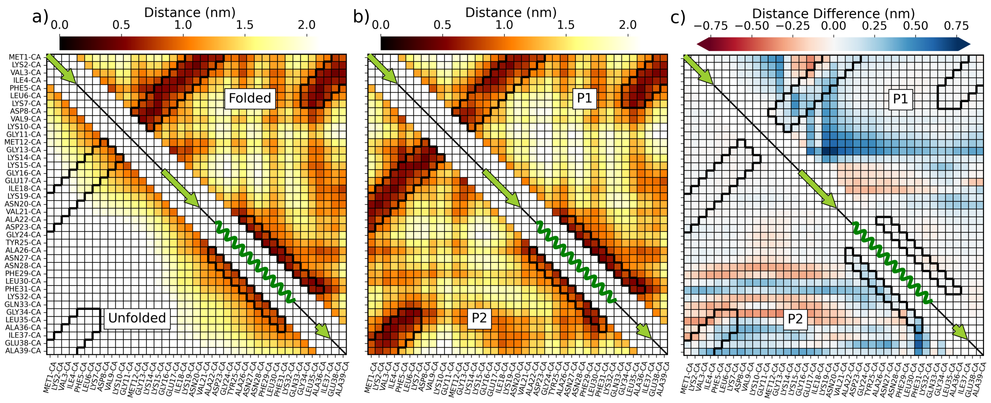


**Fig. S6** Mean distances between residues inside the interpreted structures. Panels a) and b) show the mean distances inside the structures from the folded, unfolded, P1 and P2 states and panel c) shows the distance difference between the folded state and the P1/P2 states (i.e. $d_F - d_{P1/P2}$).

To make this more comprehensible, we first describe how the propagation rules are implemented for first-order relevance attributions.

As reported in the main text (in the Methods Section), the general layer-wise propagation rule is given by

$$R_i = \sum_j \frac{q_{ij}}{\sum_i q_{ij}} \cdot R_j \ . \tag{2}$$

Without applying a particular rule, the contribution $q_{ij}$ from neuron $i$ to neuron $j$ reads

$$q_{ij} = a_i w_{ij} \ .$$

where $a_i$ is the lower-layer neuron activation and $w_{ij}$ are the weights. We can rewrite Eq. (2) as

$$R_i = a_i \sum_j \frac{w_{ij}}{z_j} \cdot R_j \ , \tag{3}$$

where $z_j := \sum_i a_i w_{ij}$ is the forward pass to neuron $j$ from the neurons $\{i\}$ of the previous layer. Since $\sum_j w_{ij} = \left[\frac{\partial}{\partial \mathbf{a}}\left(\sum_j z_j(\mathbf{a})\right)\right]_i$ with $\mathbf{a} := (a_i)_i$ denoting the vector of lower-layer activations, Eq. (3) can be written as a gradient computation

$$R_i = a_i \left[\frac{\partial}{\partial \mathbf{a}}\left(\sum_j z_j(\mathbf{a}) \cdot s_j\right)\right]_i \ , \tag{4}$$

where $s_j = R_j / z_j$ is treated as a constant. This allows us to compute the relevance attributions via efficient backpropagation, and it generalizes to different LRP-rules [26].

In this work, we utilize the generalized $\gamma$-rule [26, 27]. It is an extension of the $\gamma$-rule introduced by Montavon et. al. [26], originally, to favor positive contributions in deep neural networks with rectifier (ReLU) non-linearities. The $\gamma$-rule would simply increase the positive weights scaled by the $\gamma$-value. In our case we have smooth activation functions $a(w_{ij})$ that are non-zero for $w_{ij} < 0$. For this type of functions the generalized $\gamma$-rule is a better choice. It favors input contributions that agree with the

neuron output. This makes the gradients less noisy, improves the quality of our explanations and helps preserving the total relevance. According to the generalized $\gamma$-rule the relevance of neuron $i$ is given as

$$\begin{aligned} R_i =& \sum_j \frac{a_i^+ \cdot (w_{ij} + \gamma w_{ij}^+) + a_i^- \cdot (w_{ij} + \gamma w_{ij}^-)}{\sum_i a_i^+ \cdot (w_{ij} + \gamma w_{ij}^+) + a_i^- \cdot (w_{ij} + \gamma w_{ij}^-)} \cdot I(z_j > 0) \cdot R_j \\ &+ \sum_j \frac{a_i^+ \cdot (w_{ij} + \gamma w_{ij}^-) + a_i^- \cdot (w_{ij} + \gamma w_{ij}^+)}{\sum_i a_i^+ \cdot (w_{ij} + \gamma w_{ij}^-) + a_i^- \cdot (w_{ij} + \gamma w_{ij}^+)} \cdot I(z_j < 0) \cdot R_j \end{aligned} \tag{5}$$

with $(\cdot)^+$ and $(\cdot)^-$ denoting $\max(0, \cdot)$ and $\min(0, \cdot)$, respectively. $I(z_j > 0)$ and $I(z_j < 0)$ are functions that return the value 1 if the respective condition is satisfied and 0 otherwise. Throughout the entire analysis presented in this work, we set $\gamma := 0.1$.

We can write the denominators of (5) as

$$\sum_i a_i^+ \cdot (w_{ij} + \gamma w_{ij}^+) + a_i^- \cdot (w_{ij} + \gamma w_{ij}^-) := \sum_i d^\uparrow$$

and

$$\sum_i a_i^+ \cdot (w_{ij} + \gamma w_{ij}^-) + a_i^- \cdot (w_{ij} + \gamma w_{ij}^+) = \sum_i d^\downarrow$$

To prevent large bias values from distorting the relevance attributions, we adapt the denominators to

$$\sum_i \max\left(d^\uparrow, (w_{0j} + \gamma w_{0j}^+)\right) \tag{6}$$

and

$$\sum_i \min\left(d^\downarrow, (w_{0j} + \gamma w_{0j}^-)\right) \ , \tag{7}$$

where $w_{0j}$ is the bias value.

The general propagation rule of GNN-LRP reads

$$R_{jkl}^b = \sum_c \frac{\lambda_{jk} Q_{jk}^{bc}}{\sum_{b,j} \lambda_{jk} Q_{jk}^{bc}} R_{kl}^c \ , \tag{8}$$

where $\lambda_{ij}$ denotes the edge feature between graph nodes $i$ and $j$, and $Q_{jk}^{bc}$ is the contribution of node $j$ with its respective neuron $b$ to neuron $c$ with the associated node $k$. In practice this can be implemented by masking all nodes not directly involved in the walk of interest. For more details regarding the masking procedure please refer to [28]. The LRP-rules described above can be applied in the same manner to the higher order case. For the linear layers in the neural network model, the basic LRP rule is utilized, while for layers with non-linearities we exploit the generalized $\gamma$-rule and the bias-normalization trick described above.

As mentioned in the main text, what makes SO3Net and PaiNN stand out against SchNet are their SO3-equivariant features with angular momentum $l_{\max} > 0$. This means that SO3Net and PaiNN contain scalar feature representations ($l = 0$) and in addition to that also equivariant features of higher rotation-order up to $l_{\max}$. Equivalent to SchNet, the scalar features ($l = 0$) of PaiNN and SO3Net are embedded based on the respective atomic numbers. The equivariant features associated with $l > 0$ are initially embedded as 0-vectors. During the message passing, the equivariant features will be mixed with scalar features, and thus, influence the resulting scalar feature representation.

The models utilized in this work have the energy as an output. The forces are calculated from the first derivative of the model output with respect to the atomic positions. Since the energy is invariant with respect to rotations, the energy is predicted by a forward pass through a multilayer perceptron solely based on the invariant (scalar) features. Equivalently to previous explanations for SchNet [28, 29], we explain the predictions of PaiNN and SO3Net with respect to their scalar atomic features ($l = 0$). The reasoning for this is on the one side that the energy is predicted from the scalar features and on the other side that equivariant features are embedded as 0-vectors which would result in zero relevance attributions.

# Data Availability

Simulation data and the code to reproduce the analysis and the plots shown in the manuscript are accessible at https://box.fu-berlin.de/apps/files/?dir=/peering_inside_the_black_box_supplementary_data_and_code&fileid=555049372

# References

[1] Eastman, P. *et al.* OpenMM 7: Rapid development of high performance algorithms for molecular dynamics. *PLoS Comput. Biol.* **13**, e1005659 (2017).

[2] Chodera, J. *et al.* choderalab/openmmtools: 0.21.5 (2022). URL https://doi.org/10.5281/zenodo.6958059.

[3] Kohlmeyer, A., Vermaas, J. & Braun, E. akohlmey/topotools: Release 1.8 (2020). URL https://doi.org/10.5281/zenodo.3845031.

[4] Majewski, M. *et al.* Machine learning coarse-grained potentials of protein thermodynamics. *Nat. Commun.* **14**, 5739 (2023).

[5] Lindorff-Larsen, K., Piana, S., Dror, R. O. & Shaw, D. E. How fast-folding proteins fold. *Science* **334**, 517–520 (2011).

[6] Harvey, M. J., Giupponi, G. & De Fabritiis, G. ACEMD: Accelerating biomolecular dynamics in the microsecond time scale. *J. Chem. Theory Comput.* **5**, 1632–1639 (2009).

[7] Buch, I., Harvey, M. J., Giorgino, T., Anderson, D. P. & De Fabritiis, G. High-throughput all-atom molecular dynamics simulations using distributed computing. *J. Chem. Inf. Model.* **50**, 397–403 (2010).

[8] Piana, S., Lindorff-Larsen, K. & Shaw, D. E. How robust are protein folding simulations with respect to force field parameterization? *Biophys. J.* **100**, L47–L49 (2011).

[9] Jorgensen, W. L., Chandrasekhar, J., Madura, J. D., Impey, R. W. & Klein, M. L. Comparison of simple potential functions for simulating liquid water. *J. Chem. Phys.* **79**, 926–935 (1983).

[10] Feenstra, K. A., Hess, B. & Berendsen, H. J. C. Improving efficiency of large time-scale molecular dynamics simulations of hydrogen-rich systems. *J. Comput. Chem.* **20**, 786–798 (1999).

[11] Doerr, S. & De Fabritiis, G. On-the-fly learning and sampling of ligand binding by

high-throughput molecular simulations. *J. Chem. Theory Comput.* **10**, 2064–2069 (2014).

[12] Husic, B. E. *et al.* Coarse graining molecular dynamics with graph neural networks. *J. Chem. Phys.* **153** (2020).

[13] Wang, J. *et al.* Machine learning of coarse-grained molecular dynamics force fields. *ACS Cent. Sci.* **5**, 755–767 (2019).

[14] Ercolessi, F. & Adams, J. B. Interatomic potentials from first-principles calculations: The force-matching method. *EPL* **26**, 583 (1994).

[15] Izvekov, S. & Voth, G. A. A multiscale coarse-graining method for biomolecular systems. *J. Phys. Chem. B* **109**, 2469–2473 (2005).

[16] Noid, W. G. *et al.* The multiscale coarse-graining method. I. A rigorous bridge between atomistic and coarse-grained models. *J. Chem. Phys.* **128**, 244114 (2008).

[17] Krämer, A. *et al.* Statistically optimal force aggregation for coarse-graining molecular dynamics. *J. Phys. Chem. Lett.* **14**, 3970–3979 (2023).

[18] Schütt, K. T., Hessmann, S. S., Gebauer, N. W., Lederer, J. & Gastegger, M. Schnetpack 2.0: A neural network toolbox for atomistic machine learning. *J. Chem. Phys.* **158** (2023).

[19] Loshchilov, I. & Hutter, F. Decoupled weight decay regularization. In *ICLR* (2018).

[20] Schütt, K. T., Sauceda, H. E., Kindermans, P.-J., Tkatchenko, A. & Müller, K.-R. SchNet - a deep learning architecture for molecules and materials. *J. Chem. Phys.* **148**, 241722 (2018).

[21] Monroe, J. I. & Shell, M. S. Decoding signatures of structure, bulk thermodynamics, and solvation in three-body angle distributions of rigid water models. *J. Chem. Phys.* **151**, 094501 (2019).

[22] Stock, P. *et al.* Unraveling hydrophobic interactions at the molecular scale using

force spectroscopy and molecular dynamics simulations. *ACS Nano* **11**, 2586–2597 (2017).

[23] Chau, P.-L. & Hardwick, A. J. A new order parameter for tetrahedral configurations. *Mol. Phys.* **93**, 511–518 (1998).

[24] Errington, J. R. & Debenedetti, P. G. Relationship between structural order and the anomalies of liquid water. *Nature* **409**, 318–321 (2001).

[25] Duboué-Dijon, E. & Laage, D. Characterization of the local structure in liquid water by various order parameters. *J. Phys. Chem. B* **119**, 8406–8418 (2015).

[26] Montavon, G., Binder, A., Lapuschkin, S., Samek, W. & Müller, K.-R. Layer-wise relevance propagation: An overview. In Samek, W., Montavon, G., Vedaldi, A., Hansen, L. K. & Müller, K.-R. (eds.) *Explainable AI: Interpreting, Explaining and Visualizing Deep Learning*, 193–209 (Springer International Publishing, 2019).

[27] Andéol, L. *et al.* Learning domain invariant representations by joint wasserstein distance minimization. *Neural Networks* **167**, 233–243 (2023).

[28] Schnake, T. *et al.* Higher-order explanations of graph neural networks via relevant walks. *IEEE Trans Pattern Anal Mach Intell* **44**, 7581–7596 (2022).

[29] Letzgus, S. *et al.* Toward explainable artificial intelligence for regression models: A methodological perspective. *IEEE Signal Processing Magazine* **39**, 40–58 (2022).
